# Supplementary material for: Unified Learning from Demonstrations, Corrections, and Preferences during Physical Human-Robot Interaction
Source: arXiv:2207.03395 source file (2024-01-09)
Supplement: Supplementary file 1 [file appendix.tex]

\appendix
